# Supplementary material for: Measurements of $\pi^\pm$, K$^\pm$, p and $\bar{\textrm{p}}$ spectra in proton-proton interactions at 20, 31, 40, 80 and 158 GeV/c with the NA61/SHINE spectrometer at the CERN SPS
Source: arXiv:1705.02467 source file (2017-09-27)
Supplement: Supplementary file 1 [file AppendixA.tex]

%\clearpage
%\appendix
%\counterwithin{figure}{section}
%\section{Proof of probability method}
%\label{apendA}
%Expected value $N$ of mean multiplicity after an infinite number of trails for pions is:
%\begin{equation}
%E\left[N_{\pi}\right] = \int dm \rho_{pi}\left(m\right),
%\end{equation}
%and similarly for kaons:
%\begin{equation}
%E\left[N_{K}\right] = \int dm \rho_{K}\left(m\right),
%\end{equation}
%where $\rho\left(m\right)$ is density function. Additionally probability for given $m$ value can be defined as:
%\begin{equation}
%\omega_{K}\left( m \right) \equiv \frac{\rho_{K}\left( m \right)}{\rho\left( m \right)}, 
%\end{equation}
%where:
%\begin{equation}
%\rho\left( m \right) = \rho_{\pi}\left( m \right) + \rho_{K}\left( m \right).
%\end{equation}
%With these definitions the following relation can be shown:
%\begin{equation}
%E\left[ N_{K} \right] \equiv \int dm \rho_{K}\left( m \right) = \int dm \rho\left( m \right) \frac{\rho_{K}\left( m \right)} { \rho\left( m \right) } = \int dm \rho \left( m \right) \omega_{K}\left( m \right) \equiv E\left[ \omega_{K} \right] E\left[ N \right].
%\end{equation}
%Finally if one assumes:
%\begin{equation}
%M \equiv N_{ev} \left\langle N \right\rangle
%\end{equation}
%and $M \equiv N_{ev} \left\langle N \right\rangle$ is drawn from $\rho\left( m \right)$ and that $\omega_{K} \left( m \right)$ is given one obtains:
%\begin{equation}
%\left\langle \omega_{K} \right\rangle = \frac{1}{M} \sum_{i=1}^{M} \omega_{K}^{i} \xrightarrow[M \to \infty]{}   E\left[ \omega_{K} \right].
%\end{equation}
%Than mean multiplicity of K can then be calculated as:
%\begin{equation}
%\left\langle N_{K} \right\rangle = \left\langle \omega_{K} \right\rangle \left\langle N \right\rangle = \frac{M}{N_{ev}}
% \frac{1}{M}\sum_{i=1}^{M} \omega_{K}^{i} = \frac{1}{N_{ev}}\sum_{i=1}^{M}\omega_{K}^{i}.
%\end{equation}
%Finally the calculation shows that the proposed method allows to obtain the mean multiplicity of a given particle type:
%\begin{equation}
%\left\langle N_{K} \right\rangle = \frac{1}{N_{ev}}\sum_{i=1}^{M}\omega_{K}^{i} \xrightarrow[M \to \infty]{}   E\left[ N_{K} \right].
%\end{equation}
%In this method one also assumes that relative particle yields do not change across a bin.
